# Supplementary material for: Struct-MDC: Mesh-Refined Unsupervised Depth Completion Leveraging Structural Regularities from Visual SLAM
Source: arXiv:2204.13877 source file (2022-04-29)
Supplement: Supplementary file 1 [file appendix.tex]

\section*{APPENDIX}

% 깃랩링크
